# Supplementary material for: Impact of inter-city interactions on disease scaling
Source: arXiv:2501.01395 source file (2025-01-02)
Supplement: Supplementary file 1 [file supplementary.pdf]

# Impact of inter-city interactions on disease scaling

**Nathalia A. Loureiro[1], Camilo R. Neto[1], Jack Sutton[2], Matjaž Perc[3,4,5,6], and Haroldo V. Ribeiro[7,*]**

[1]Complex Systems Modeling Program, School of Arts, Sciences and Humanities, University of São Paulo, São Paulo, Brazil
[2]College of Science and Engineering, University of Derby, Markeaton Street, Derby DE22 3AW, United Kingdom
[3]Faculty of Natural Sciences and Mathematics, University of Maribor, Koroška cesta 160, 2000 Maribor, Slovenia
[4]Community Healthcare Center Dr. Adolf Drolc Maribor, Vošnjakova ulica 2, 2000 Maribor, Slovenia
[5]Complexity Science Hub Vienna, Josefstädterstraße 39, 1080 Vienna, Austria
[6]Department of Physics, Kyung Hee University, 26 Kyungheedae-ro, Dongdaemun-gu, Seoul, Republic of Korea
[7]Departamento de Física, Universidade Estadual de Maringá, Maringá, PR 87020-900, Brazil
[*]Correspondence to hvr@dfi.uem.br

## Supplemental Materials

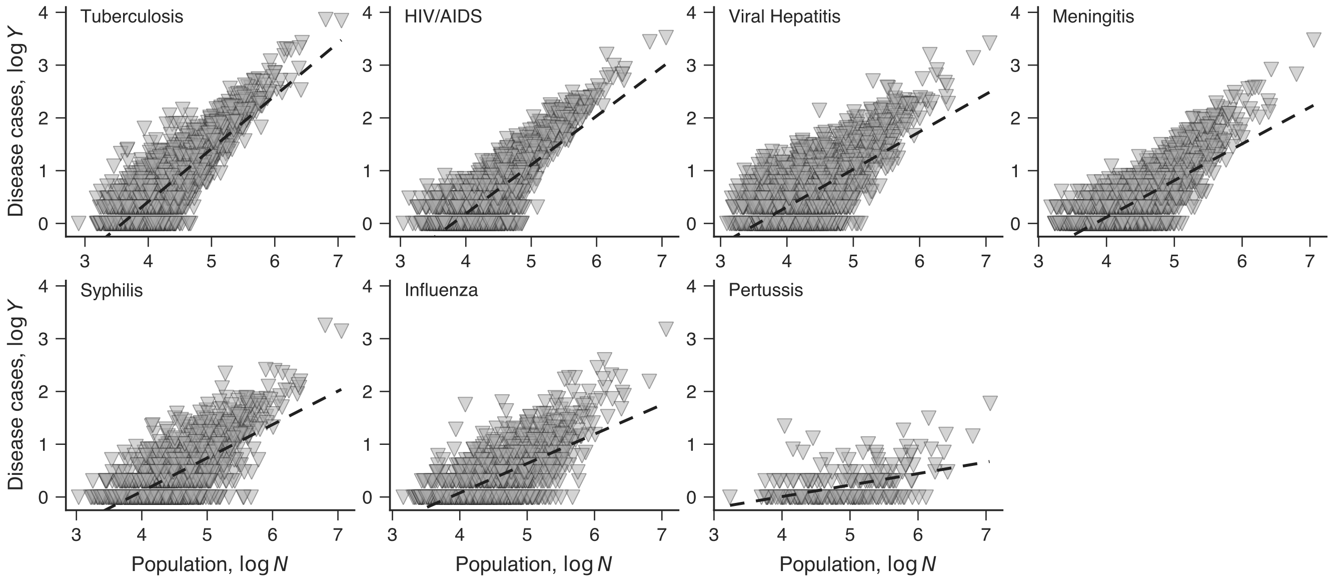


**Figure S1.** Scaling laws between disease cases and population. The panels show the relationship between reported cases and city population for each of the seven infectious diseases in our dataset. Disease names are indicated within each panel, with dashed lines representing the urban scaling model (Eq. 1 in the main text) adjusted for each disease.

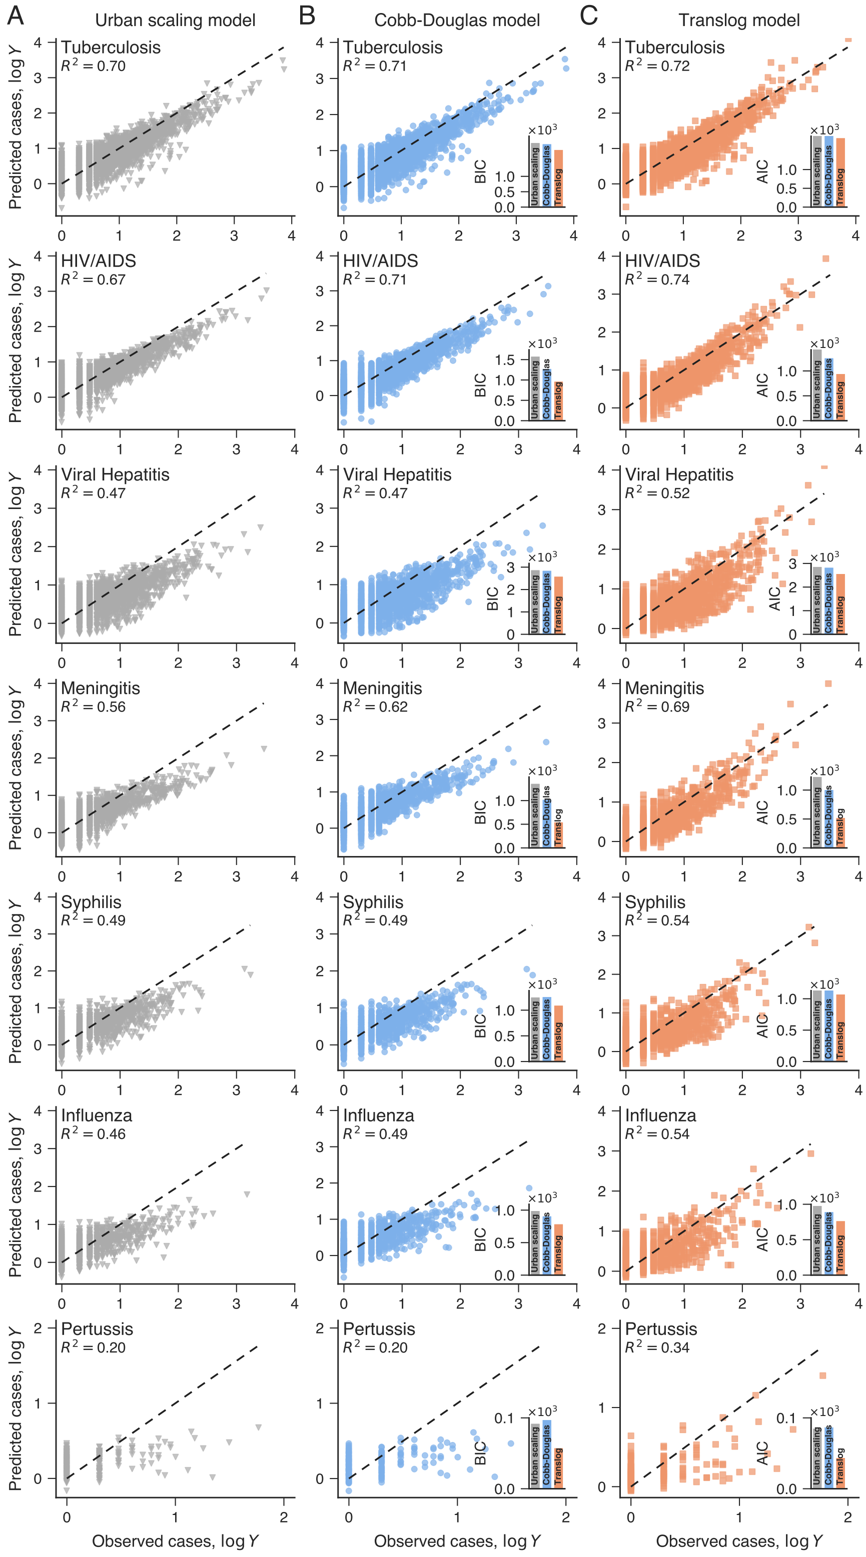


**Figure S2.** Comparison of urban scaling predictions with enhanced descriptions from the Cobb-Douglas and translog models across all disease types in our dataset. Panels (A), (B), and (C) compare the predictions from the urban scaling (Eq. 1), Cobb-Douglas (Eq. 2), and translog (Eq. 3) models for all disease types. Disease cases are expressed on a base-10 logarithmic scale with dashed lines representing the identity function. Insets in panels (B) and (C) present the Bayesian information criterion (BIC) and Akaike information criterion (AIC) calculated for each model. Additionally, the coefficients of determination ($R^2$) are shown within each plot.

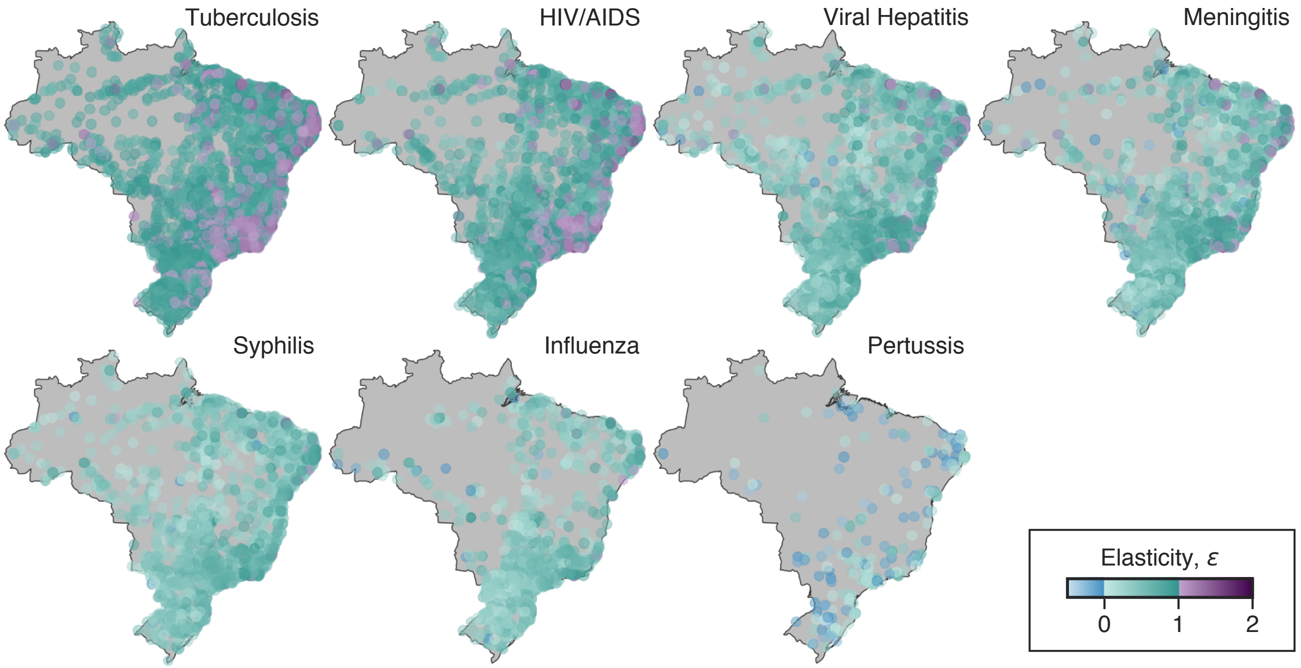


**Figure S3.** Spatial distributions of the elasticity of scale. Maps show the spatial distribution of the elasticity of scale ($\varepsilon$) estimated using the translog model (Eq. 4 in the main text) for each of the seven infectious diseases in our dataset. Color-coded markers represent the $\varepsilon$ values and the locations of cities reporting cases of each disease type.

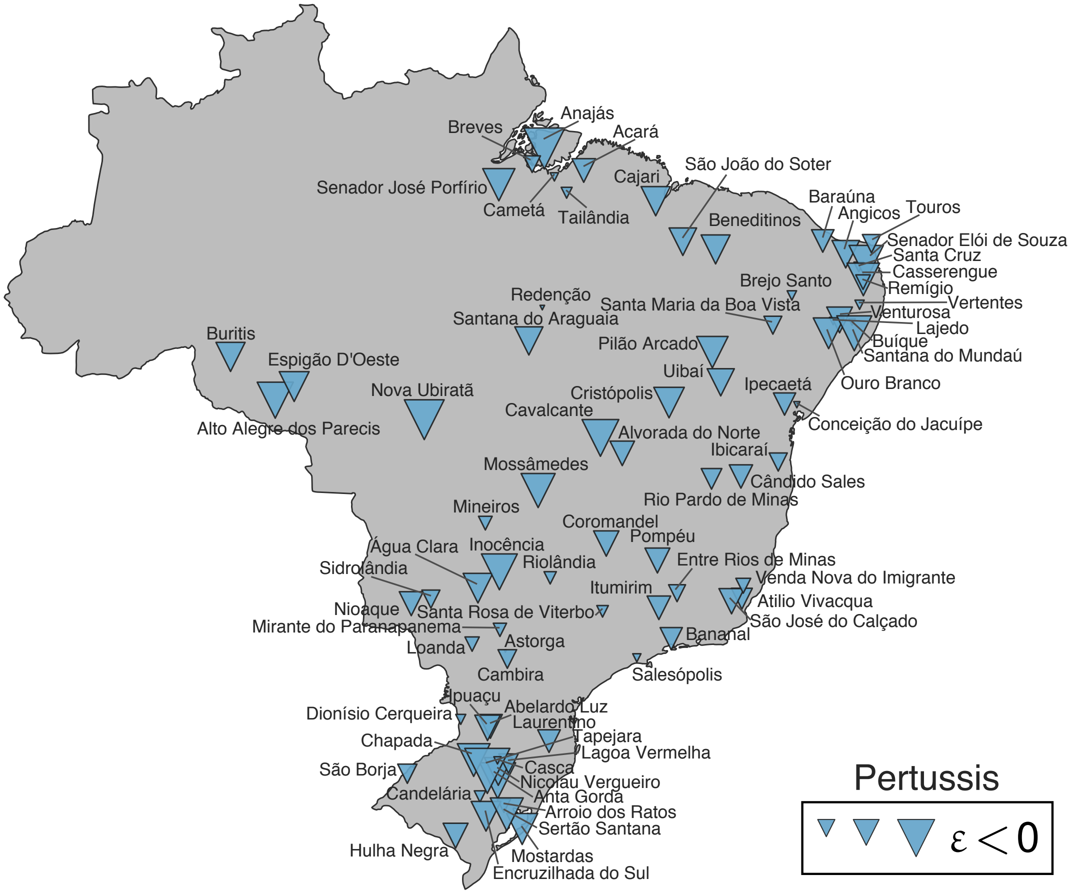


**Figure S4.** Cities displaying negative elasticity of scale for pertussis. The markers on the map indicate the location of each Brazilian city reporting negative elasticity of scale for pertussis. The size of the markers is proportional to the absolute values of the elasticity of scale $\varepsilon$. Figure created using Matplotlib and GeoPandas.
